# Supplementary material for: Charge order in LuFe2O4: an unlikely route to ferroelectricity
Source: arXiv:1112.0978 source file (2012-05-03)
Supplement: Supplementary file 1 [file Supplementary.pdf]

# Supplementary Information to:
# "Charge order in $LuFe_2O_4$: an unlikely route to ferroelectricity"

**Authors:** J. de Groot, T. Mueller, R. A. Rosenberg, D. J. Keavney, Z. Islam, J.-W. Kim, and M. Angst

In this supplement, we provide additional details of our XMCD measurements. In Fig. S1a, the x-ray absorption spectra (XAS) are for right and left circular light and for both the magnetic-field configuration with $H$ parallel and anti parallel to $c_{\mathrm{Hex}}$ presented. Experimental artifacts and non-magnetic contributions can sometimes contribute to the XMCD signal, so taking the four spectra is a way of correcting for those. As for a purely magnetic XMCD signal expected, the observation for $\Delta\mu(H) = \mu_+(H) - \mu_-(H)$ is identical within error bars to $\Delta\mu(-H) = \mu_-(-H) - \mu_+(-H)$. In the $L_3$-region of the TEY-XAS (Fig. S1a), the $Fe^{3+}$ peak is higher than the $Fe^{2+}$ peak suggesting an $Fe^{3+}$ contribution of more than 50%. Because TEY has a very short probing depth and because the structure refinement and other bulk-sensitive techniques (e.g. Mössbauer spectroscopy [1]) clearly show a $Fe^{2+}$: $Fe^{3+}$ ratio close to $1:1$, this is most likely an effect of surface oxidation (our crystals were cleaved ex-situ in normal atmosphere). Indeed, the peak ratio is close to the one shown in [2], who cleaved their crystals in $5 \cdot 10^{-8}$ mbar, whereas crystals cleaved in higher vacuum of $7 \cdot 10^{-10}$ mbar [3] resulted in peaks closer in height. To verify this, we measured also XAS and XMCD in fluorescence yield (Fig. S1b), which is more bulk-sensitive. Indeed, the $Fe^{2+}$: $Fe^{3+}$ peakratio in the $L_3$-region is close to $1:1$ in fluorescence yield. Strong self-absorption (well visible in the changed $L_3$: $L_2$ intensity ratio) results in a somewhat noisy XMCD signal in fluorescence-yield, but despite of this the main feature of the XMCD, a large downward peak at the $Fe^{2+}$ position and a smaller ($\sim$50%) upward peak at the $Fe^{3+}$ position is clearly visible also in fluorescence-yield; confirming its bulk nature (Fig. S1b). In addition, we note that the (better-statistics) XMCD-signal in TEY (Fig. S1a) is extremely similar to the XMCD-signal [3] (the green curve in Fig. S1a) obtained on crystals cleaved in ultra-high vacuum, further confirming the bulk-nature.

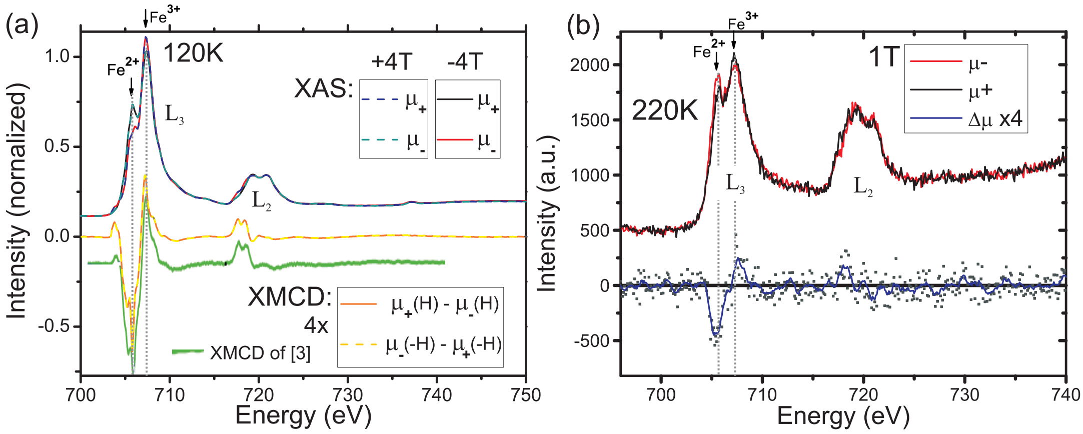


FIG. S1: (a) The four XAS spectra at the Fe $L_{2/3}$ edges, taken with $\pm 4\,\mathrm{T}\ ||c_{\mathrm{Hex}}$ and with RCP and LCP light. The signal was obtained from the total electron yield (TEY) channel. For comparison the scaled XMCD result of [3] is additionally presented. (b) The two XAS spectra in 1 T measured with RCP and LCP light, obtained from the total fluorescence yield (TFY) channel. Furthermore, the XMCD signal between both the XAS curves is shown, indicating the bulk behavior of the TEY signal. For better comparison with the TEY signal, the solid blue line is the five points smoothed TFY-XMCD signal.

The main feature in XMCD, a downward peak at the $Fe^{2+}$ and a smaller upward peak at the $Fe^{3+}$ position directly implies that the net magnetic moment of the $Fe^{2+}$-sites is in field-direction and a net moment of the $Fe^{3+}$ sites points to the opposite direction. Because the spin-value of $Fe^{3+}$ is larger than the one of $Fe^{2+}$, the considerably smaller XMCD intensity at the $Fe^{3+}$ position implies that fewer $Fe^{3+}$ spins are aligned antiparallel to field than $Fe^{2+}$ spins are aligned $||H$. This is consistent with the local valence-specific spin configuration proposed in both [3] and [2]. Together with

TABLE S1: Possible $Fe^{2+}$ and $Fe^{3+}$ spin configurations according to the measured XMCD signal. The magnetic moments of $Fe^{2+}$ and $Fe^{3+}$ are given in brackets. Here, the $4.7\,\mu_B$ spin-moment plus orbital magnetic moment on $Fe^{2+}$ and the pure spin-moment on $Fe^{3+}$ of $5.0\,\mu_B$ are used.

| № | $Fe^{2+}$ ($4.7\,\mu_B$) | № | $Fe^{3+}$ ($5.0\,\mu_B$) |
|---|---|---|---|
| 1 | ↑ ↑ ↑ ↑ ↑ ↑ | 1* | ↓ ↓ ↓ ↓ ↓ ↑ |
| 2 | ↑ ↑ ↑ ↑ ↑ ↓ | 2* | ↓ ↓ ↓ ↓ ↑ ↑ |
| 3 | ↑ ↑ ↑ ↑ ↓ ↓ | | |

the well-known magnetic saturation moment of $\sim 3\,\mu_B$/f.u. and two facts of the recently published spin-model from neutron diffraction [4] we can readily show that this is indeed the only possible local valence-specific spin configuration. The first fact, that the magnetic and crystallographic cell are equal [4], implies that there are only 12 Fe-sites (i.e. 6 each 3+ and 2+), and the second fact, that this is an Ising-system with all sites fully ordered implies that each site contributes parallel or antiparallel. From the above direct implications of the XMCD, this leaves only three possible arrangements, tabulated in Tab. S2. All other combination of Tab. S1 are inconsistent with the XMCD implication that more $Fe^{2+}$ spin moments are parallel to the field than $Fe^{3+}$ are antiparallel.

Here, № $(1+2^*)$ is the only combination of local spin environments, which gives a reasonable net moment of $3.03\,\mu_B$/f.u., very close to the measured saturation moment of $\sim 3\,\mu_B$/f.u. found in literature [4–6], which is also valid for the sample used in this work. All other combinations of possible spin configurations in Tab. S2, will result in much lower overall net moments (the next highest is № $(2+2^*)$ and № $(1+1^*)$ both with $\sim 1.4\,\mu_B$/f.u., all others combinations have negative values), and therefore can be excluded. Furthermore, № $(1+2^*)$ to be the favored local spin configuration does not depend strongly on the actual $Fe^{2+}$ and $Fe^{3+}$ moments. By changing the total $Fe^{2+}$ magnetic contribution to $4\,\mu_B$/f.u. and the $Fe^{3+}$ moment to $5\,\mu_B$/f.u., or both valences equal to $4.5\,\mu_B$/f.u., the solution № $(1+2^*)$ is still the configuration which is the closest to the observed saturation moment.

TABLE S2: Magnetic saturation moment of the three local spin configurations according Tab. S1.

| Combination | $\mu_B$/f.u. |
|---|---|
| № $(1+2^*)$ | 3.03 |
| № $(2+2^*)$ | 1.46 |
| № $(1+1^*)$ | 1.36 |


[1] X. S. Xu *et al.*, Phys. Rev. Lett. **101**, 227602 (2008).
[2] K. Kuepper *et al.*, Phys. Rev. B. **80**, 220409(R) (2009).
[3] K.-T. Ko *et al.*, Phys. Rev. Lett. **103**, 207202 (2009).
[4] J. de Groot *et al.*, Phys. Rev. Lett. **108**, 037206 (2012).
[5] W. Wu *et al.*, Phys. Rev. Lett. **101**, 137203 (2008).
[6] J. Iida *et al.*, J. Phys. Soc. Jpn. **62**, 1723 (1993).
